# Supplementary material for: Nonlinear dynamics of Aharonov-Bohm cages
Source: arXiv:1810.07641 source file (2019-03-12)

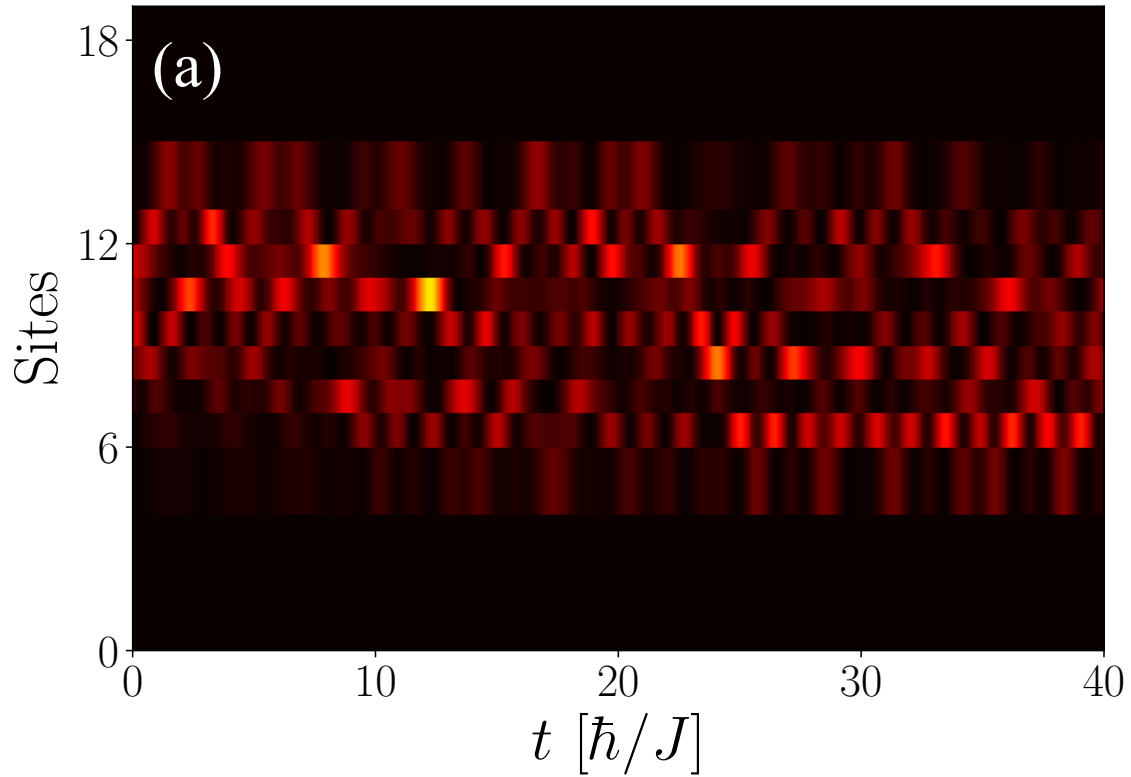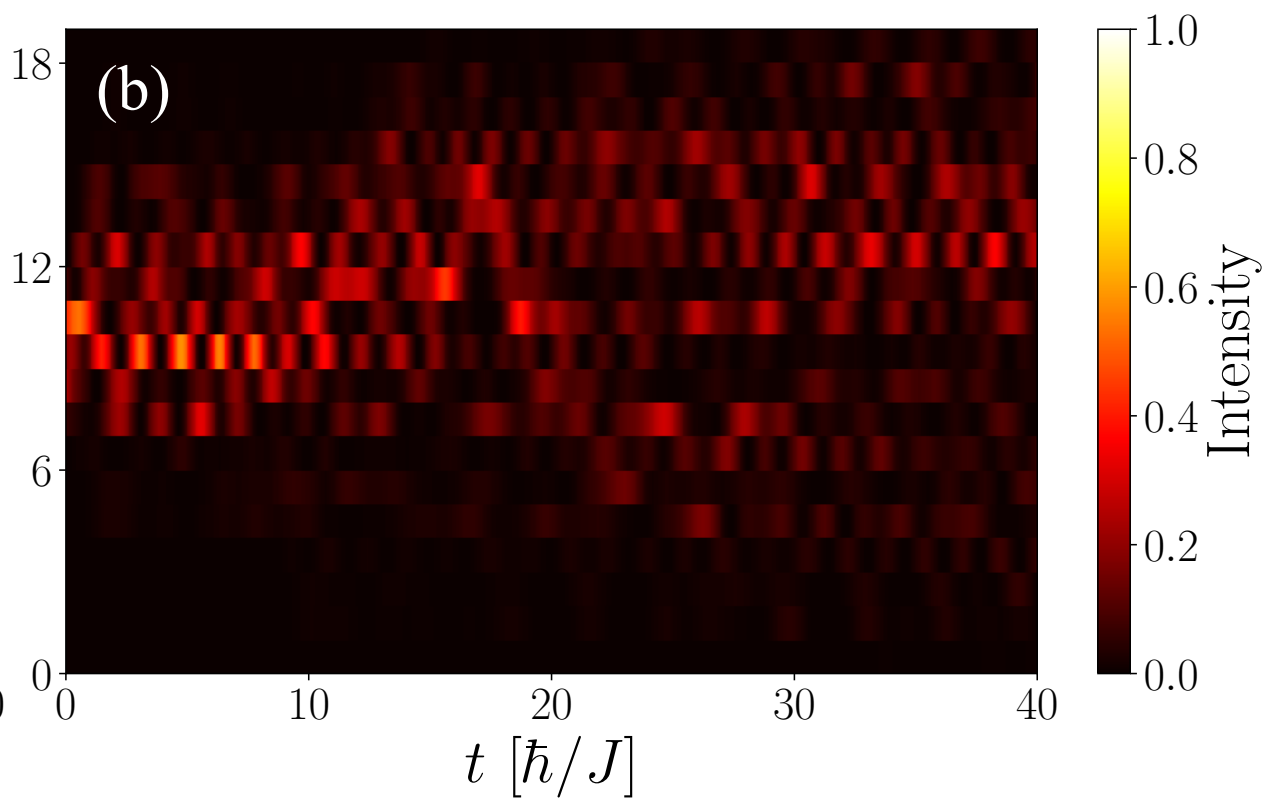

(a)

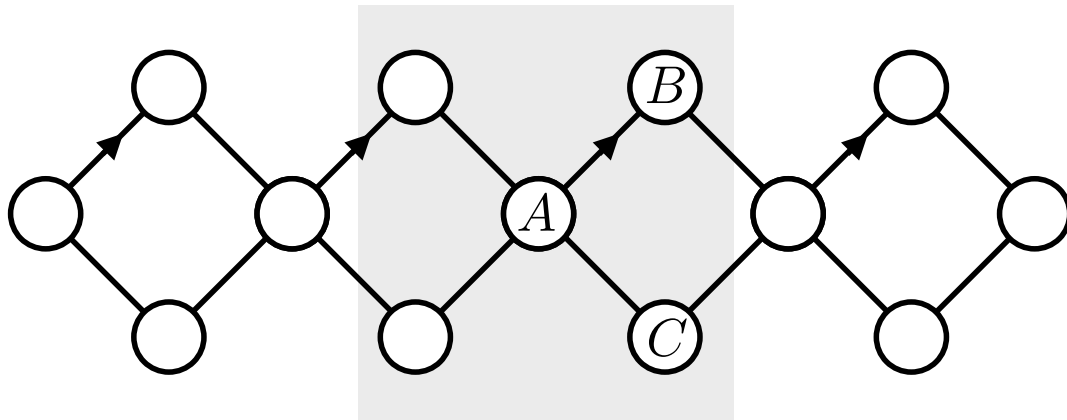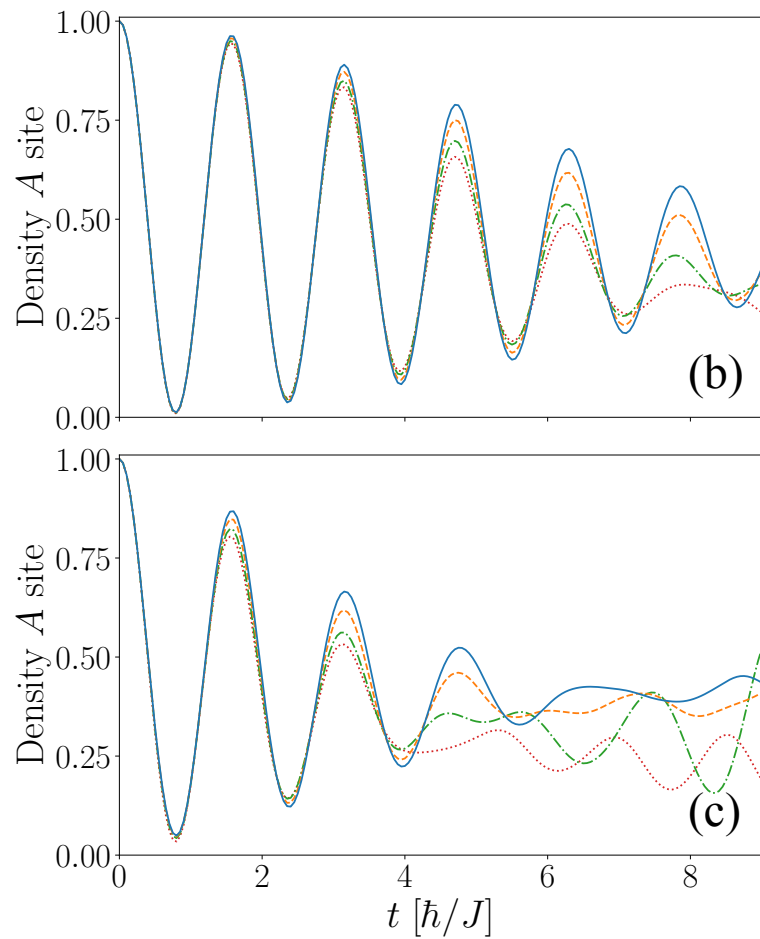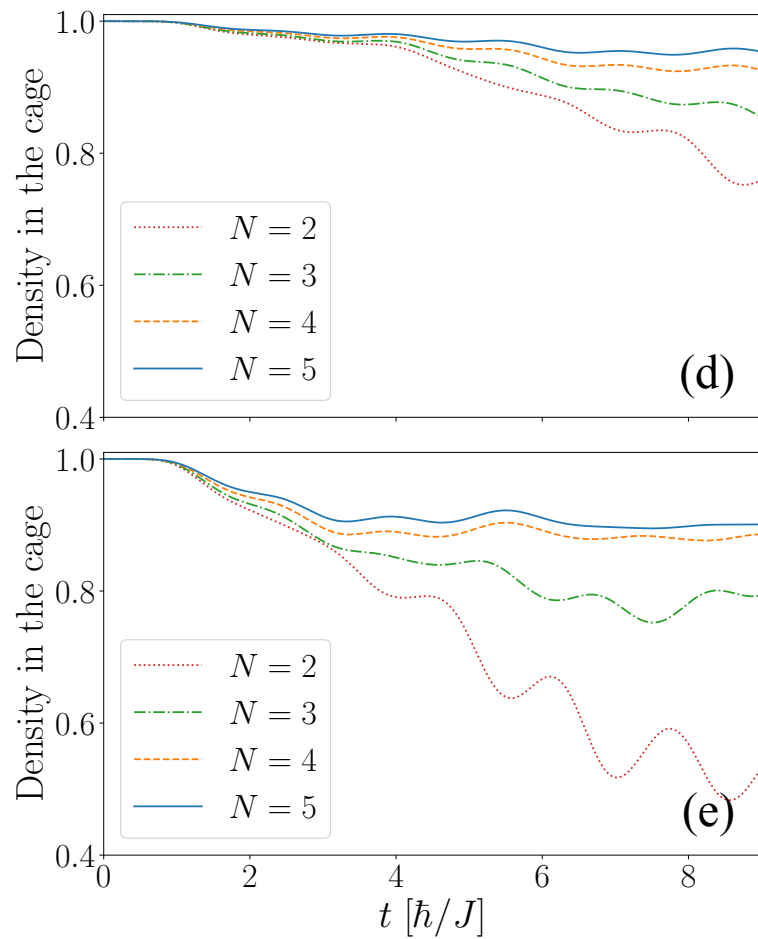

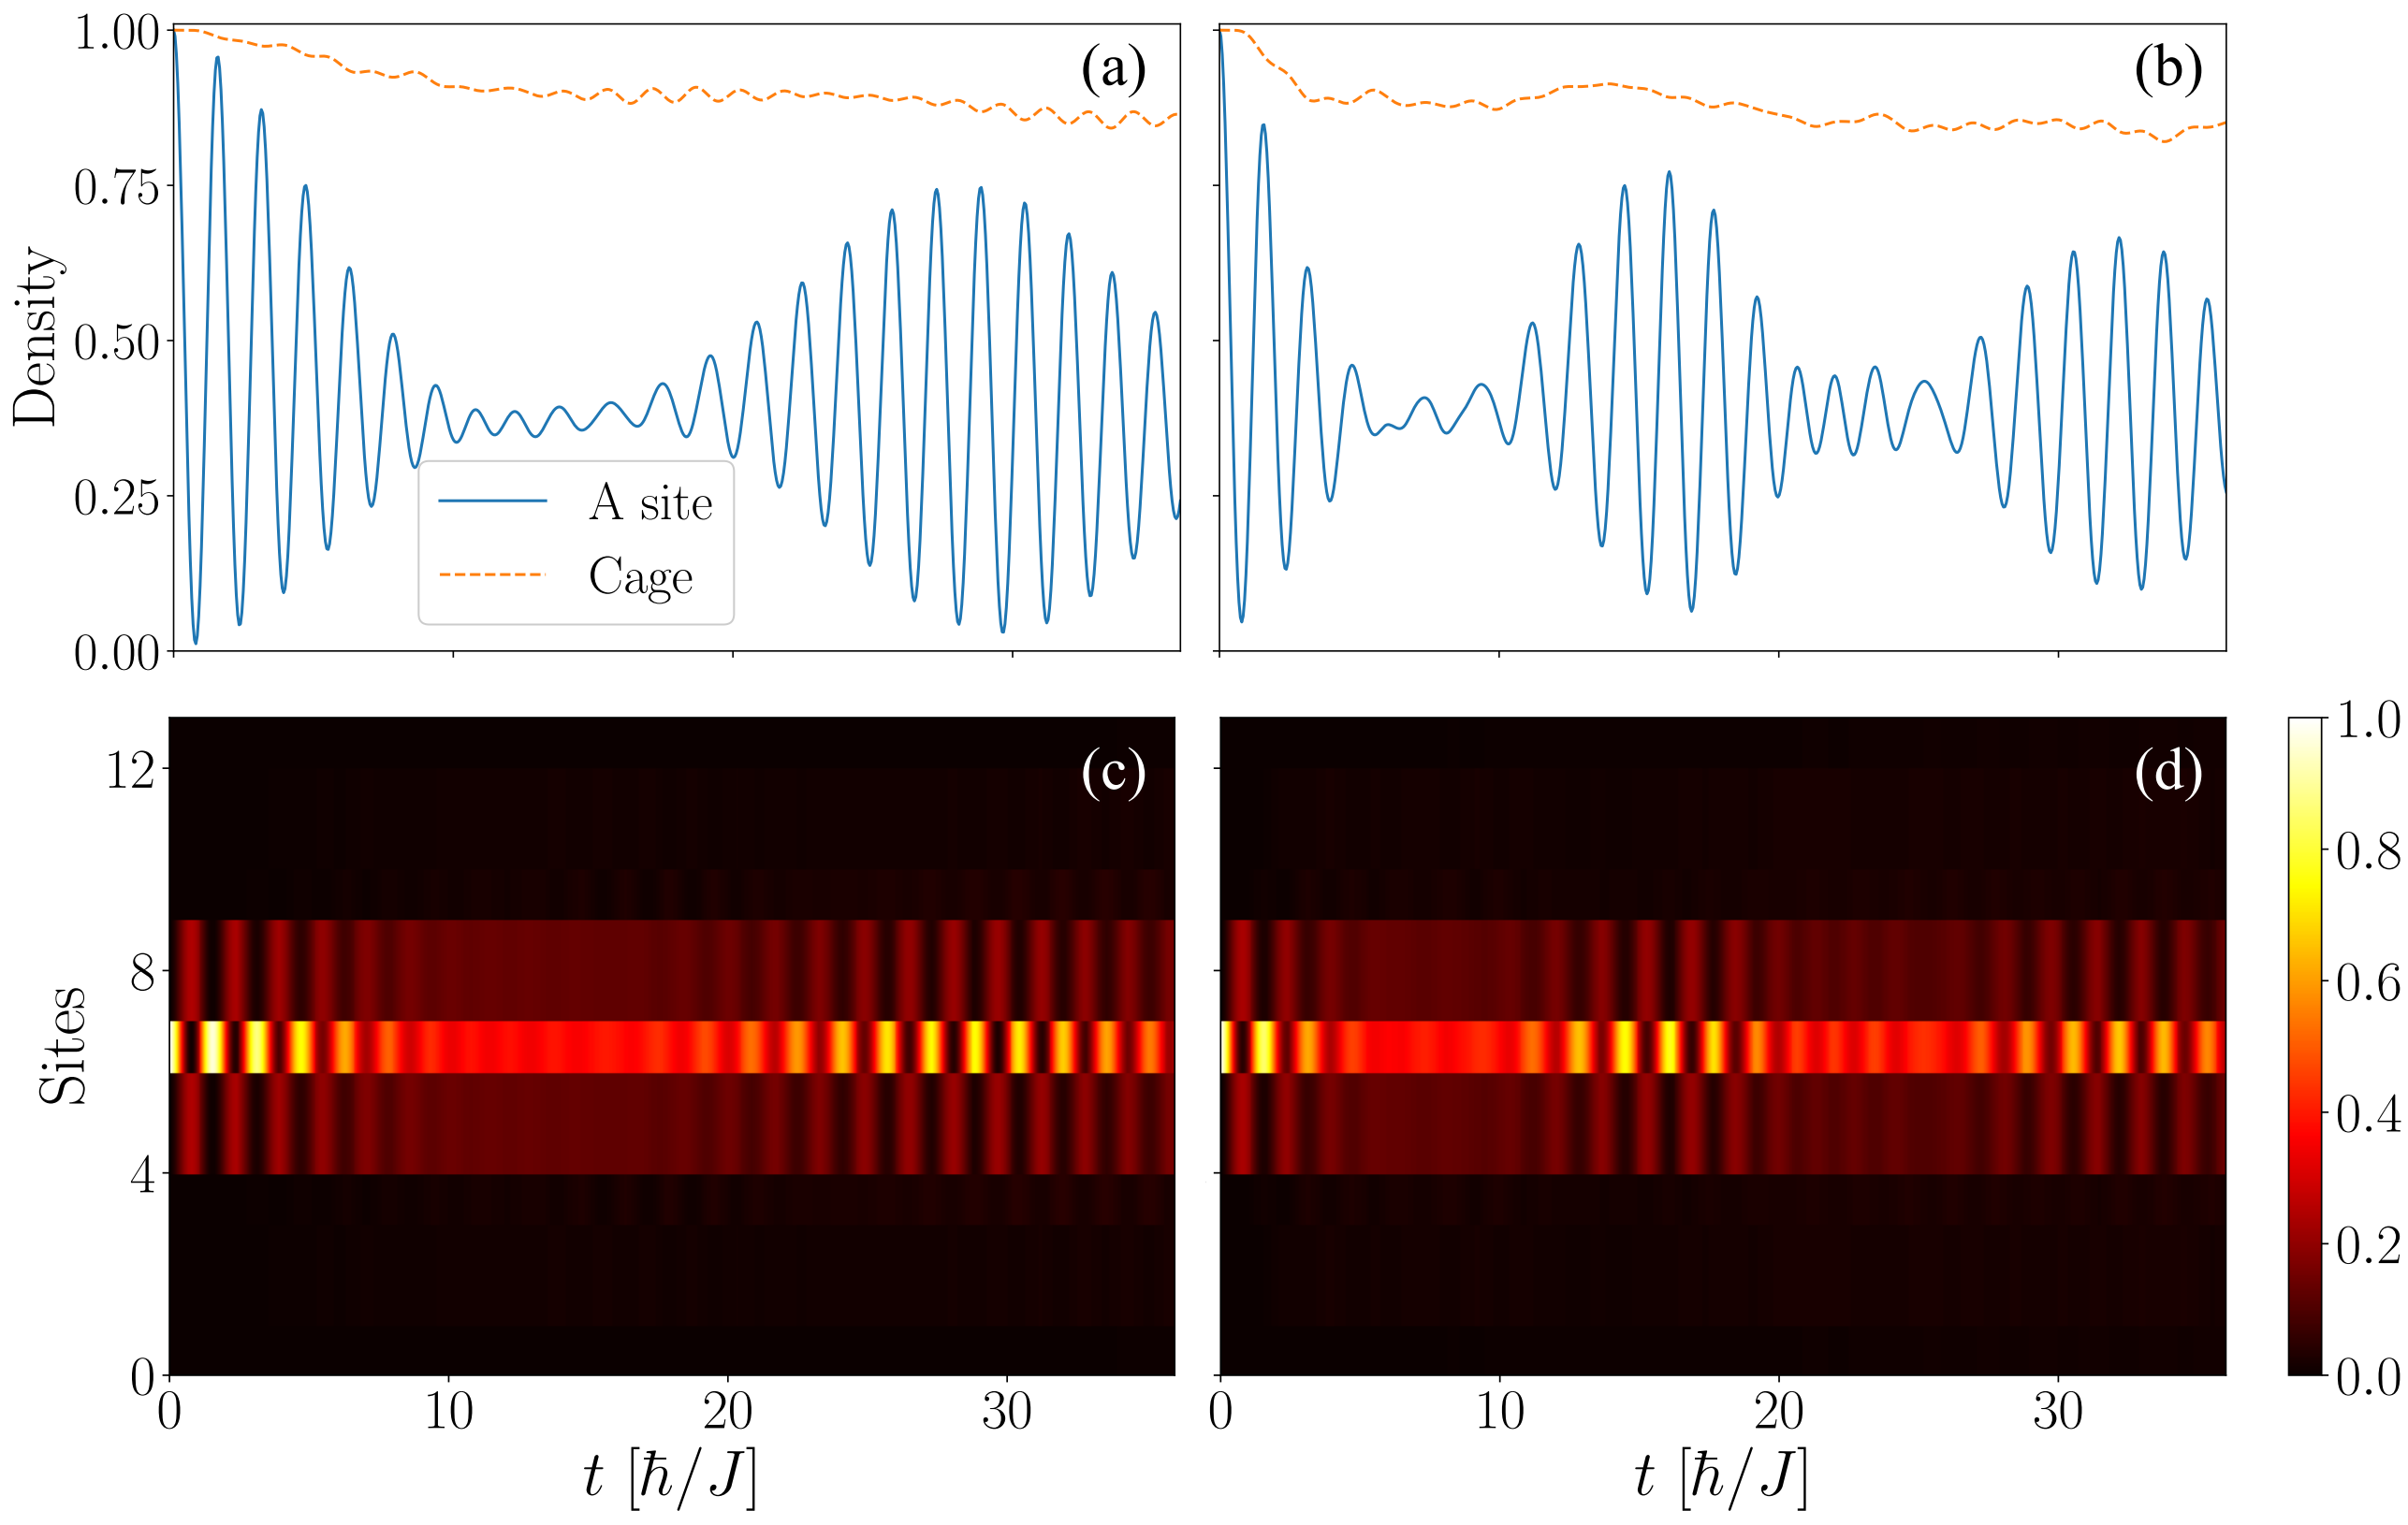

Supplement: Supplementary file 1 [file Fig1_SM.pdf]
